# Supplementary material for: Orientation and dynamics of stiff polymeric nanoparticles
Source: arXiv:1801.07976 ancillary file (2018-01-24)
Supplement: Supplementary file 1 [file flow_stop_letter_supplemental_information.pdf]

# Orientation and dynamics of stiff polymeric nanoparticles - Supplemental Information

Christophe Brouzet,* Nitesh Mittal, L. Daniel Söderberg, and Fredrik Lundell

*Linné FLOW Centre, KTH Mechanics,*

*KTH Royal Institute of Technology, Stockholm SE-100 44, Sweden and*

*Wallenberg Wood Science Centre, KTH Royal*

*Institute of Technology, Stockholm SE-100 44, Sweden*

(Dated: January 24, 2018)

* brouzet@mech.kth.se

## EXPERIMENTAL SET-UP

Figure S1 shows the experimental set-up used in this study, recently introduced by Rosén *et al.* [1].

It is composed of a flow-focusing channel, made of 4 branches having a square cross-section with $h = 1$ mm sides. The CNC or CNF suspension is shown in gray while the water sheath flows are in blue. The flow is produced using syringe pumps (NE-4000, New Era Pump Systems, Inc.), with a flow rate $Q_c = 23.4$ ml/hr for the suspension and a combined flow rate of $Q_s = 27$ ml/hr for the sheath flows.

In order to stop the flow, one 3-way solenoid-driven slider valve (MTV-3SL Series, Takasago Electric, Inc.) is located at the end of each branch of the channel. The ”common” way C is connected to the ”normally open” way NO and allows the flow to go from the syringe pumps to the channel and from the channel to the dump. By applying a strong electric current, the connection of the ”common” way C switches almost immediatly from the ”normally open” way NO to the ”normally closed” way NC, deviating the flow directly

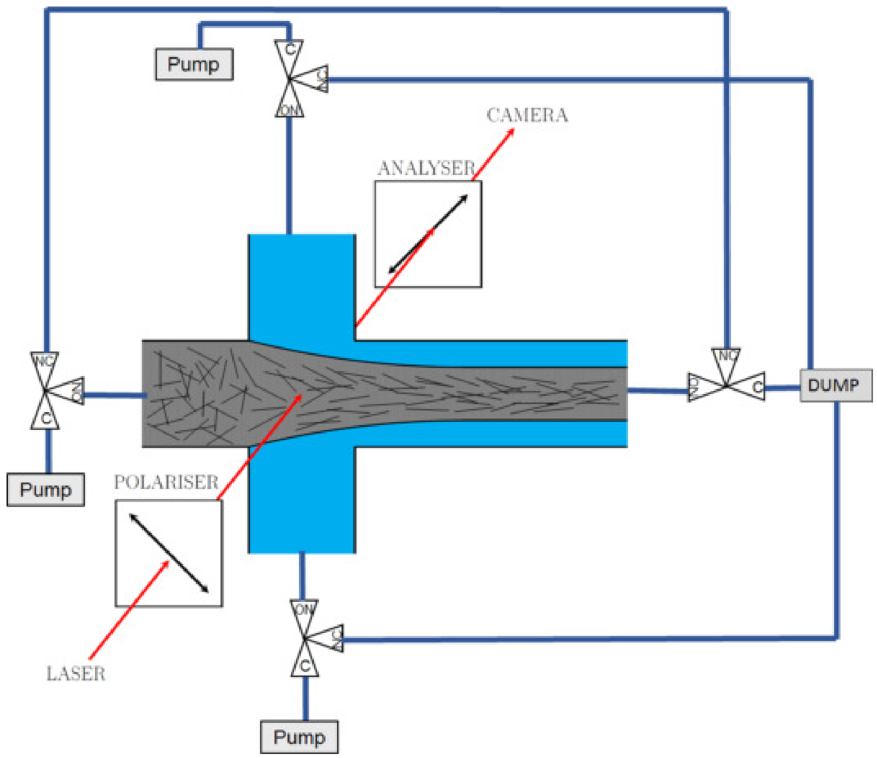


FIG. S1. Schematic of the experimental set-up, adapted from Rosén *et al.* [1].

to the dump without passing through the channel. The channel is therefore isolated and the flow inside is viciously stopped.

The birefringence set-up is sketched with the two crossed polarisers, having polarising directions at 45° with respect to the flow direction. A red laser light passes through the system and is collected by a high-speed camera (SpeedSense M, Dantec Dynamics). The recorded intensity $I$ is then given by

$$I = I_0 \sin\left(\frac{2\pi e \Delta n}{\lambda}\right)^2, \tag{1}$$

where $I_0$ is a constant which depends on the laser intensity, $e$ the thickness of the sample crossed by the light, $\Delta n$ the birefringence and $\lambda$ the wavelength of the light. As $I_0$ cannot be measured, we define $B = I^{1/2} \propto \Delta n$ for small $\Delta n$. In the main body of the paper, the quantity $B$ is also called birefringence by extension.

For both the suspensions (CNC and CNF), the presented results are based on an average of 10 consecutive experiments to reduce noise. When comparing individual experiments for all cases, they show good reproducibility. The camera is used to record 3000 images at 5000 fps for the CNC and 31000 images at 1000 fps for the CNF with approximately 1000 images recorded before the flow is stopped. The time to stop the flow is found to be sufficiently small compared to the frame rate of the camera.

## PREPARATION OF CNC AND CNF

CNC were prepared according to the following procedure. 20 g of a never-dried dissolving pulp (from Domsjö Fabriker AB, Örnsköldsvik, Sweden) was dispersed in $H_2SO_4$ (175 ml, 64 wt%) and immersed in an oil bath preheated at 45°C for 45 minutes under rigorous magnetic stirring. Thereafter, the reaction mixture was diluted ten times with deionized water. The CNC were thoroughly washed through repeated centrifugation and re-dispersion cycles then dialyzed against deionized water for ten days. Subsequently, CNC were dispersed by ultrasonication with an amplitude of 28% using pulse function (5 s pulse on and 2 s pulse off) for 30 minutes. Finally, the CNC suspension was filtered on glass filter pore 1 to remove any large aggregates.

CNF were prepared from chemically bleached wood fibers (a mixture of 60% Norwegian spruce and 40% Scots pine, provided by Domsjö AB, Sweden). The wood pulp fibers were

chemically treated with a 2,2,6,6-tetramethylpiperidinyl-1-oxyl (TEMPO)-mediated oxidation reactions previously reported elsewhere [2]. In brief, cellulose pulp fibers (1 g) were suspended in 0.05M sodium phosphate (Sigma Aldrich) buffer (90 ml, pH 6.8) dissolving TEMPO (16 mg, 0.1 mmol) and sodium chlorite (Sigma Aldrich) (80%, 1.13 g, 10 mmol). The 2M sodium hypochlorite solution (0.5 mL) after dilution to 0.1M with the 0.05M sodium phosphate buffer was added to the suspension. The suspensions were stirred at 500 rpm for 1 hour. The TEMPO-oxidized pulp fibers were washed thoroughly with deionized water by filtration. After the chemical pre-treatment, aqueous suspensions of the fibers were passed through a high-pressure homogenizer. At the end of this, CNF suspensions, with a concentration higher than 5 g/l were obtained. In an additional step, the unfibrillated and agglomerated fiber bundles were removed from the CNF suspensions. The gel like suspensions were diluted by adding deionized water, mixed thoroughly using a mechanical mixer (12000 rpm for 10 min, Ultra Turrax, IKA, Germany) and sonication (10 min, Sonics Vibracell, USA). The diluted suspensions were then centrifuged at 5000 rpm for 60 minutes followed by the removal of precipitates and the supernatants were used for further studies. The dry content of the suspensions was determined by gravimetric analysis.

The surface charges of the CNC (103 $\mu$eq/g) and CNF (380 $\mu$eq/g) were determined by polyelectrolyte titration using a Stabino particle charge mapping equipment with streaming potential measurements (ParticleMetrix, Germany). Dispersions (0.5 ml, 0.1 wt%) were diluted to a total volume of 10 ml and titrated with pDADMAC with a molecular weight of $400 - 500$ kDa and a total charge of 0.351 $\mu$eq/ml.

## MEASUREMENTS OF THE LENGTH AND THE WIDTH OF THE SAMPLES

The length of CNF and CNC were measured using transmission electron microscopy (TEM) (JEOL JEM-1400 TEM) at an accelerating voltage of 120 kV. Images were acquired with a Ruby camera following "systematic, uniform, random" rule to avoid bias. Prior observation, the sample was deposited on a carbon coated copper grid treated with glow discharge and stained with 2% uranyl acetate solution. Typical TEM images for CNC and CNF are shown in Fig. 1 of the main body of the paper.

The diameter of CNF were measured using atomic force microscopy (AFM) (MultiMode 8, Bruker, Santa Barbara, CA, USA), assuming that all fibrils are cylindrical. Therefore the

height measured with the AFM corresponds directly to the diameter of the CNF. Oxidation of silicon wafers (Addison Engineering Inc., San José, CA, US) were carried out at 1000°C for 1 hr for the formation of silica layer. The wafers were washed with ethanol and milli-Q followed by drying and treatment in the plasma chamber (PCD 002, Harrick Scientific Corp., Ossining, NY, US) for 5 min to make the surface hydrophilic. Wafers in the size of $5 \times 5$ mm were dipped in the CNF suspensions and left to dry in air at room temperature. The diameter of CNC were measured directly from the high resolution TEM images.

## DIFFUSION COEFFICIENT FOR A POLYDISPERSE SUSPENSION OF RODS

Here we describe how to reach Eq. (4) of the main body of the text starting from the results of Marrucci and Grizzuti [3, 4] and one main assumption. We consider a rod of length $L$ in a semi-dilute and polydisperse suspension. Using integrals rather than discrete summations, the diffusion coefficient of such rod is given by [3, 4]

$$D_r(L) = \frac{\beta k_B T}{\eta L^4} \frac{1}{\int_0^{+\infty} \tilde{c}(L')L'Q(L,L')\mathrm{d}L' \left( \int_0^L \tilde{c}(L')L'^4 Q(L,L')\mathrm{d}L' + L^3 \int_L^{+\infty} \tilde{c}(L')L'Q(L,L')\mathrm{d}L' \right)}, \tag{2}$$

where $\beta$ is a numerical factor, $k_B$ the Boltzmann constant, $T$ the temperature, $\eta$ the viscosity of the solvent, $\tilde{c}$ the concentration distribution of the rods depending on $L$ and $Q$ anisotropic corrections depending on the orientation of rods having a length $L$ and $L'$. We assume

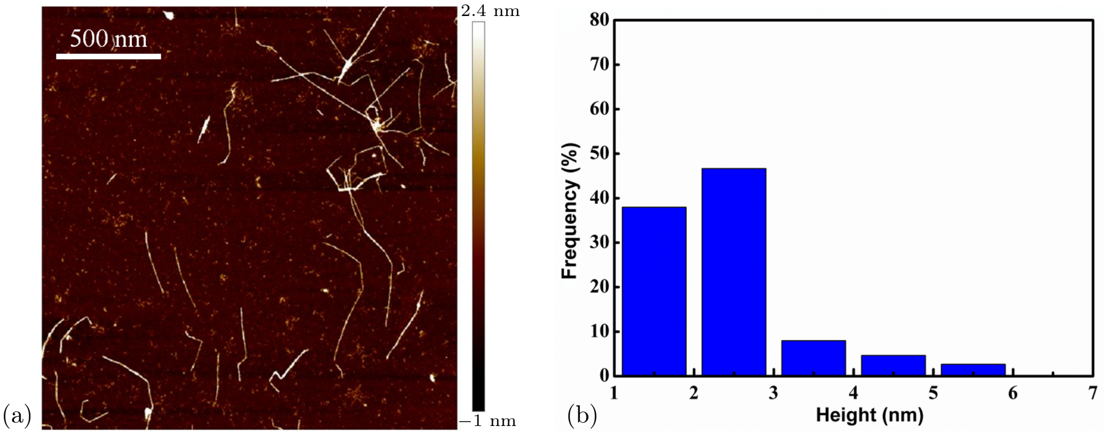


FIG. S2. (a): Typical AFM image for CNF. The colorbar indicates the height measured by the AFM. (b): Histogram of the height (i.e. diameter) of 200 individual CNF.

that the anisotropic corrections are negligible, because the system is always far from full alignment. This means that $Q \approx 1$ and leads to

$$D_r(L) = \frac{\beta k_B T}{\eta L^4} \frac{1}{\int_0^{+\infty} \tilde{c}(L')L'\mathrm{d}L' \left(\int_0^L \tilde{c}(L')L'^4\mathrm{d}L' + L^3 \int_L^{+\infty} \tilde{c}(L')L'\mathrm{d}L'\right)}, \tag{3}$$

$$= \frac{\beta k_B T}{\eta L^4} \frac{L_*^2}{\left(\int_0^L \tilde{c}(L')L'^4\mathrm{d}L' + L^3 \int_L^{+\infty} \tilde{c}(L')L'\mathrm{d}L'\right)}, \tag{4}$$

$$= \frac{\beta k_B T L_*^4}{\eta L^7} \frac{\int_0^{+\infty} \tilde{c}(L')L'\mathrm{d}L'}{\left(\int_0^L \tilde{c}(L')L'(L'/L)^3\mathrm{d}L' + \int_L^{+\infty} \tilde{c}(L')L'\mathrm{d}L'\right)}, \tag{5}$$

$$= \frac{\beta k_B T L_*^4}{\eta L^7} \Gamma(L), \tag{6}$$

with $L_* = \left(\int_0^{+\infty} \tilde{c}(L')L'\mathrm{d}L'\right)^{-1/2}$ and

$$\Gamma(L) \equiv \frac{\int_0^{+\infty} \tilde{c}(L')L'\mathrm{d}L'}{\left(\int_0^L \tilde{c}(L')L'(L'/L)^3\mathrm{d}L' + \int_L^{+\infty} \tilde{c}(L')L'\mathrm{d}L'\right)}. \tag{7}$$

The factor $\Gamma(L)$ depends on the length $L$ of the rod but also on the concentration distribution $\tilde{c}$ of the rods at different lengths, related to the length distribution shown in Fig. 1(b) of the main paper. The factor $\Gamma$ is plotted as a function of the rod length $L$ in Fig. S3, for the length distribution of the CNF suspension used in this paper. For the smallest rods, we can see that $\Gamma$ tends to 1, in agreement with the limit of $L \to 0$ in Eq. (7). However, $\Gamma$ increases with the length $L$ and reaches its maximum for the largest rods ($L = 1350$ nm) around 4.5, remaining therefore of order 1. This allows us to neglect the factor $\Gamma$ when the expression of the rotary diffusion coefficient $D_r$ is used to convert the time scales $\{\tau_j\}$ into the length scales $L$ in the main body of the paper. Indeed, the power 7 over the length $L$ is much more dominant that the small correction introduces by the factor $\Gamma$ here. The conversion is thus valid, provided the anisotropic corrections are small. This is indeed the only hypothesis needed to perform these calculations.

Neglecting anisotropic corrections simplifies the problem twice. First, analytical calculations for the diffusion coefficient are possible without knowing the orientation state of the fibrils, allowing us to obtain the diffusion coefficient for a given length. Second, this decouples the de-alignment dynamics of each rod. Indeed, under this approximation, the diffusion coefficient of a rod having a length $L$ depends only on $L$ and the length distribution. Thus, it is constant during all the relaxation towards isotropy. If the anisotropic

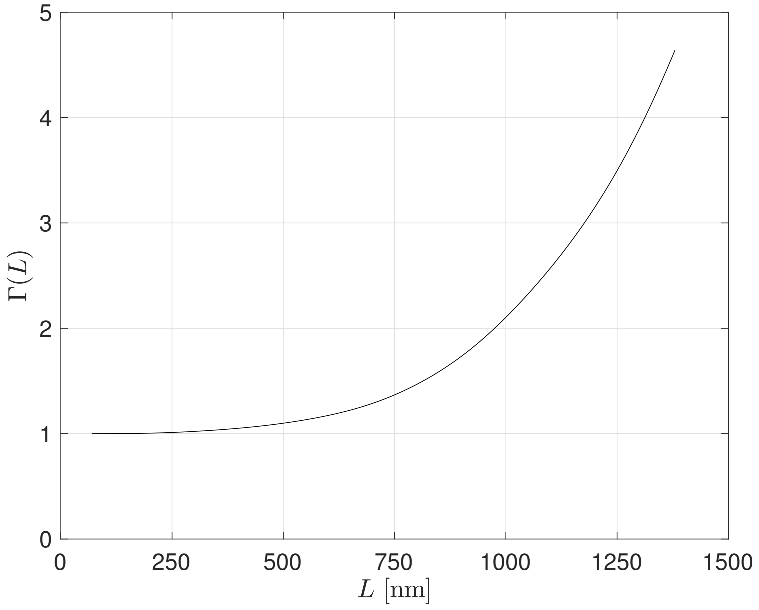


FIG. S3. Correction factor $\Gamma$ as a function of the length of the rod $L$.

corrections are not any more negligible, this introduces a coupling between the lengths: the diffusion coefficient of a rod having a length $L$ now depends also on the orientation states of all fibres in the suspension. As these orientation states change with time due to relaxation towards isotropy, this introduces a time dependency for the diffusion coefficient, invalidating the inverse Laplace transform approach made in the main body of the paper.

Anisotropic corrections to the diffusion coefficient are described theoretically by Doi and Edwards [5] for the monodisperse case and by Marrucci and Grizzuti [3, 4] for the polydisperse case. Experimentally, these corrections are difficult to evaluate because the birefringence is a quantitative measure of only the average orientation and not the full orientation density function. However, this function can be obtained using other techniques, like small-angle X-ray scattering (SAXS) for example [1]. In the flow-focusing channel, the orientation density function is not fully peaked, meaning that the system is not completely aligned [1]. Therefore, anisotropic corrections remain relatively small and are negligible. Consequently, the isotropic approximation made in the main body of the paper is totally valid in our case.

## ERROR BARS AND STABILITY OF THE INVERSE LAPLACE TRANSFORM

Following Rogers *et al.* [6], the stability of the inverse Laplace transform within the measurement noise has been evaluated. The inverse Laplace transform used in the main body of the paper has been achieved with 20 time scales, spread in the range $[5t_{\mathrm{min}}; 5t_{\mathrm{max}}]$, with $t_{\mathrm{min}}$ the time interval between two images and $t_{\mathrm{max}}$ the duration of the full acquisition. By changing the different parameters of the fit, i.e. minimal and maximal time scales considered and the number of time scales, several distributions $B^0(L)$ can be obtained and compared, providing error bars. Inverse Laplace transforms have been performed with 2 other minimal times scales, $3t_{\mathrm{min}}$ and $10t_{\mathrm{min}}$, with 2 other maximal time scales, $3t_{\mathrm{max}}$ and $10t_{\mathrm{max}}$, and with 2 other numbers of time scales, 10 and 30. Only one parameter has been varied at a time, the others being fixed to the standard inverse Laplace transform (20 time scales in the range $[5t_{\mathrm{min}}; 5t_{\mathrm{max}}]$). This thus provides 6 different distributions $B^0(L)$, in addition to the one obtained with the standard procedure. All the distributions obtained are very similar leading to small error bars. They typically have the size of the symbols used to represent the distributions and are therefore not plotted in Fig. 4 in the main body of the paper.

---


[1] T. Rosén, N. Mittal, S. V. Roth, P. Zhang, L. D. Söderberg, and F. Lundell, arXiv:1801.07558v1.

[2] A. Isogai, T. Saito, and H. Fukuzumi, Nanoscale **3**, 71 (2011).

[3] G. Marrucci and N. Grizzuti, J. Polym. Sci., Polym Lett. Ed. **21**, 83 (1983).

[4] G. Marrucci and N. Grizzuti, J. Non-Newtonian Fluid Mech. **14**, 13 (1984).

[5] M. Doi and S. F. Edwards, *Oxford Science Publications* (1986).

[6] S. S. Rogers, P. Venema, L. M. C. Sagis, E. van der Linden, and A. M. Donald, Macromolecules **38**, 2948–2958 (2005).
